# Supplementary material for: Mixed Policy Gradient: off-policy reinforcement learning driven jointly by data and model
Source: arXiv:2102.11513 source file (2024-02-24)
Supplement: Supplementary file 1 [file addi_results.tex]

\section{Additional results}\label{appendix.addi_results}
Fig. \ref{fig.error} graphs the tracking errors of all baseline algorithms on the path tracking task. We calculate the tracking errors using the root mean squared over states of 5 episodes every 3000 iterations (each episode has a fixed length of 200). Specifically, the errors are calculated by
\begin{equation}
\nonumber
\text{Error}_{\dagger} = \sqrt{\mathbb{E}_{\dagger\in\mathbb{C}_{\dagger}}\left\{(\dagger - \dagger_{\text{ref}})^2\right\}}
\end{equation}
where $\text{Error}_{\dagger}, \dagger \in \{y, \phi, u\}$ is to denote the position error, heading angle error and velocity error, respectively. $\mathbb{C}_{\dagger}$ is the corresponding state collection of 5 episodes.
\begin{figure}[h]
\centering
\captionsetup[subfigure]{justification=centering}
\subfloat[Position error]{\label{fig.position_error}\includegraphics[width=0.4\textwidth]{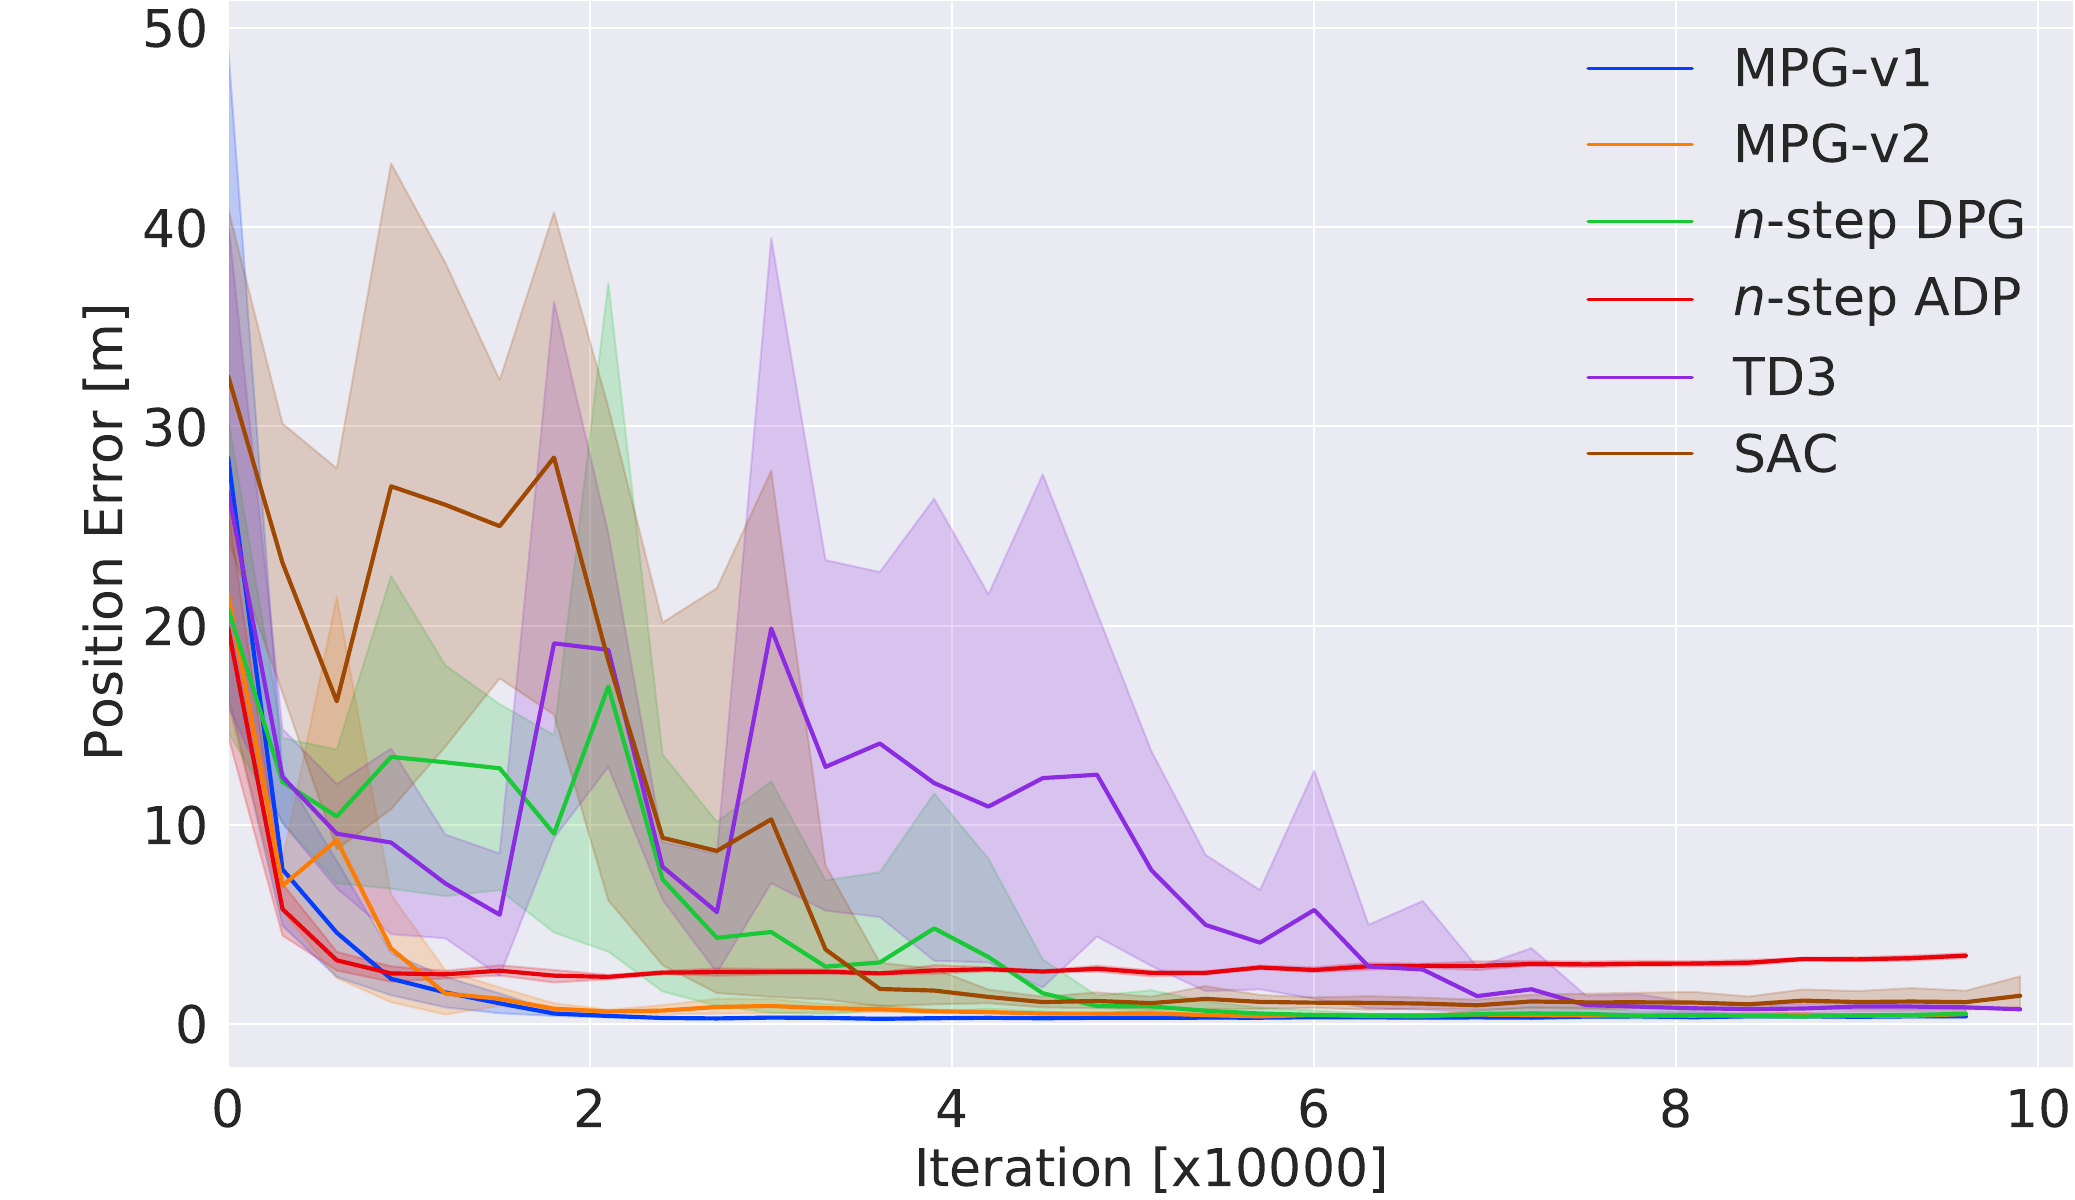}}\\
\subfloat[Heading angle error]{\label{fig.heading_angle_error}\includegraphics[width=0.4\textwidth]{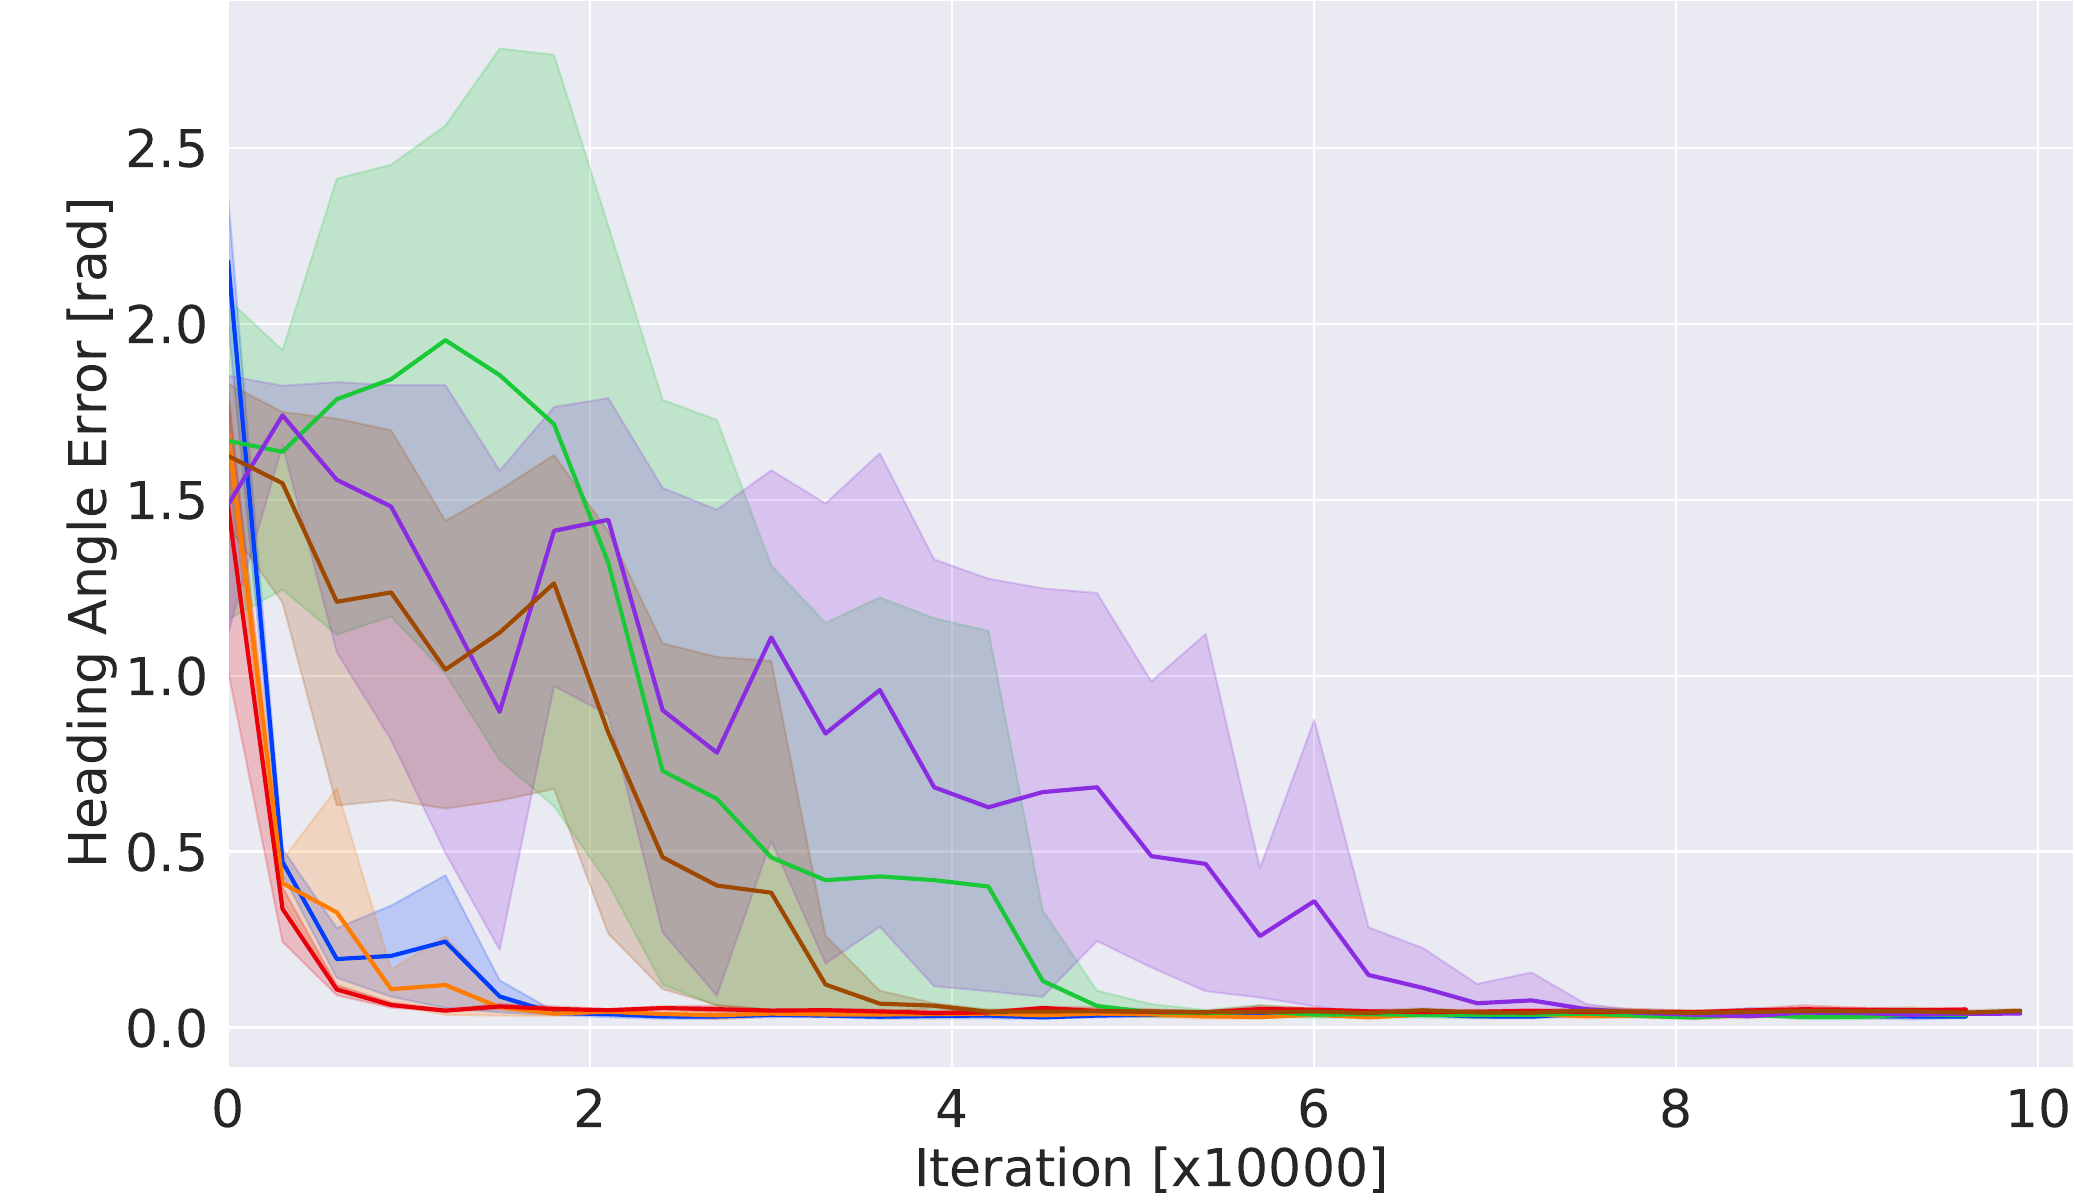}}\\
\subfloat[Velocity error]{\label{fig.velocity_error}\includegraphics[width=0.4\textwidth]{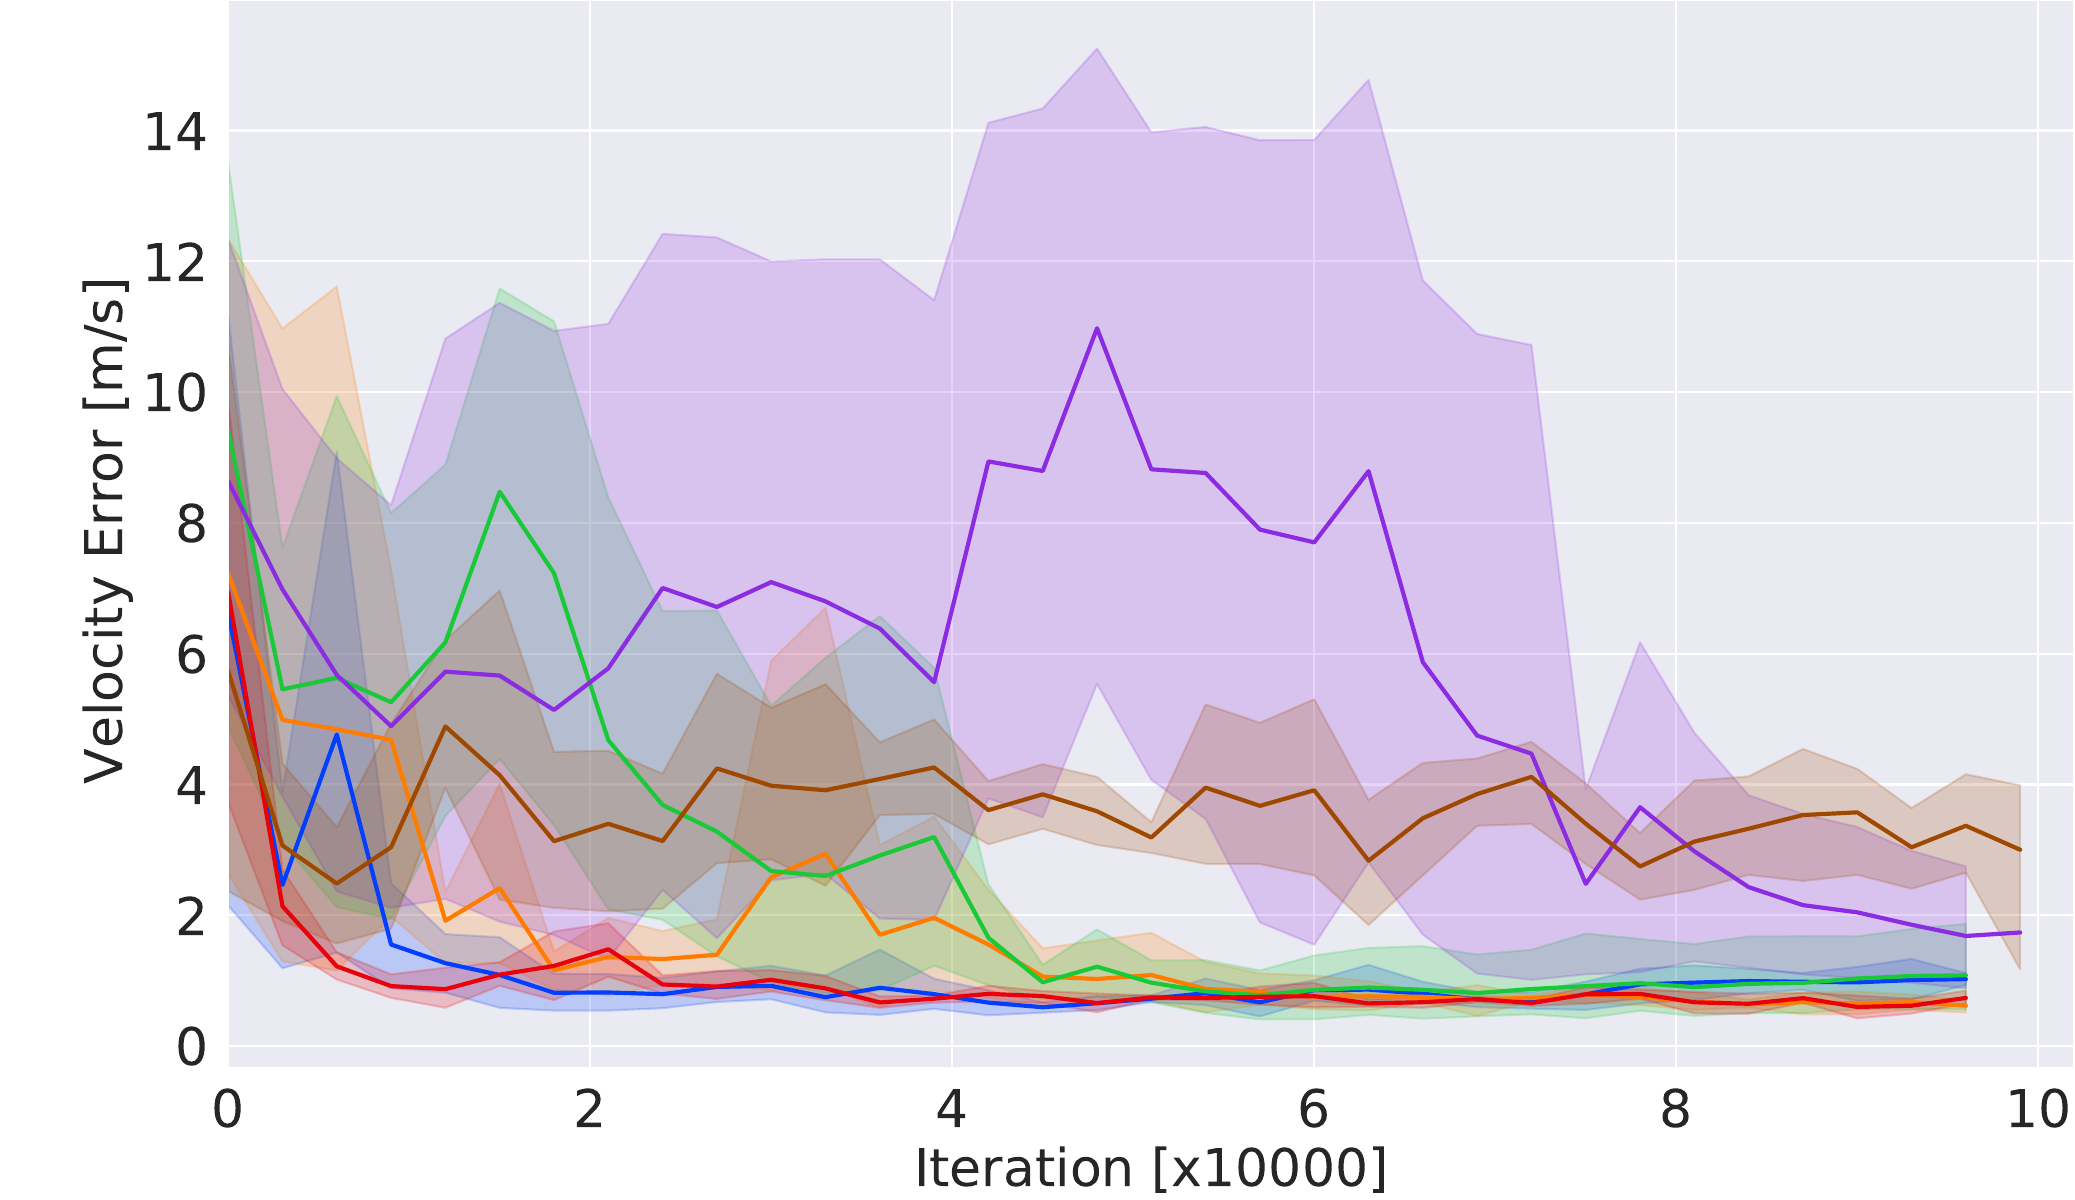}}
\caption{Tracking errors of path tracking task. (a) Position error. (b) Heading angle error. (c) Velocity error. The solid lines correspond to the mean and the shaded regions correspond to 95\% confidence interval over 5 runs.}
\label{fig.error}
\end{figure}

\newpage
Besides, Fig. \ref{fig.cart_pole_error} graphs the state magnitudes on the inverted pendulum task, which is calculated by the root mean square over actions of 5 episodes every 3000 iterations. Specifically, the state magnitudes are calculated by
\begin{equation}
\nonumber
\text{State}_{\dagger} = \sqrt{\mathbb{E}_{\dagger\in\mathbb{C}_{\dagger}}\left\{\dagger^2\right\}}
\end{equation}
where $\text{State}_{\dagger}, \dagger \in \{x, \Dot{x}, \theta, \Dot{\theta}\}$ is to denote the magnitude of the cart position, cart velocity, pole angle and pole angular velocity, respectively. $\mathbb{C}_{\dagger}$ is the corresponding state collection of 5 episodes.

\newpage
\quad
\begin{figure}[!htbp]
\centering
\captionsetup[subfigure]{justification=centering}
\subfloat[Cart position]{\label{fig.cart_position}\includegraphics[width=0.4\textwidth]{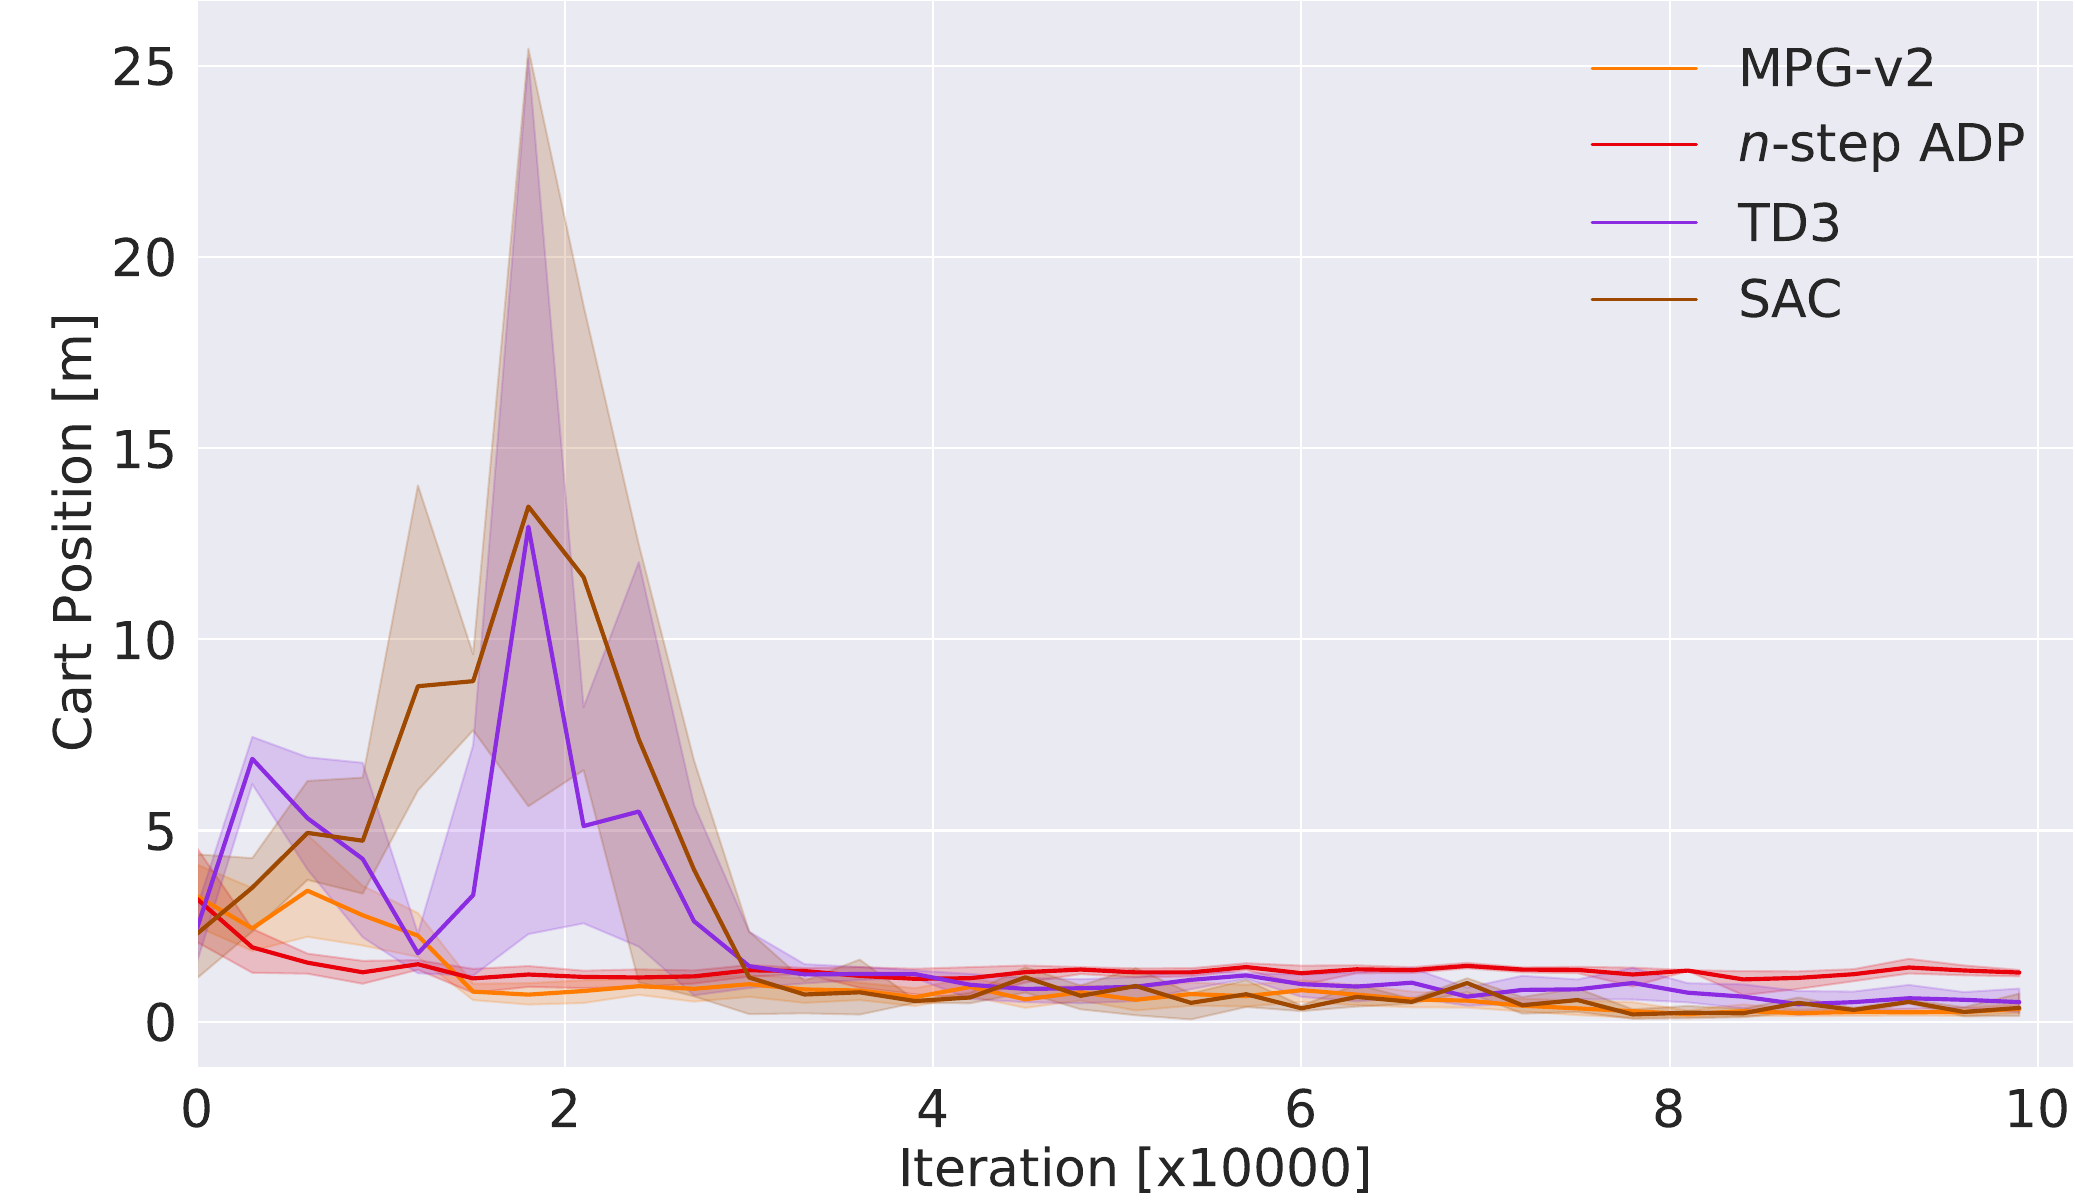}}\\
\subfloat[Cart velocity]{\label{fig.cart_velocity}\includegraphics[width=0.4\textwidth]{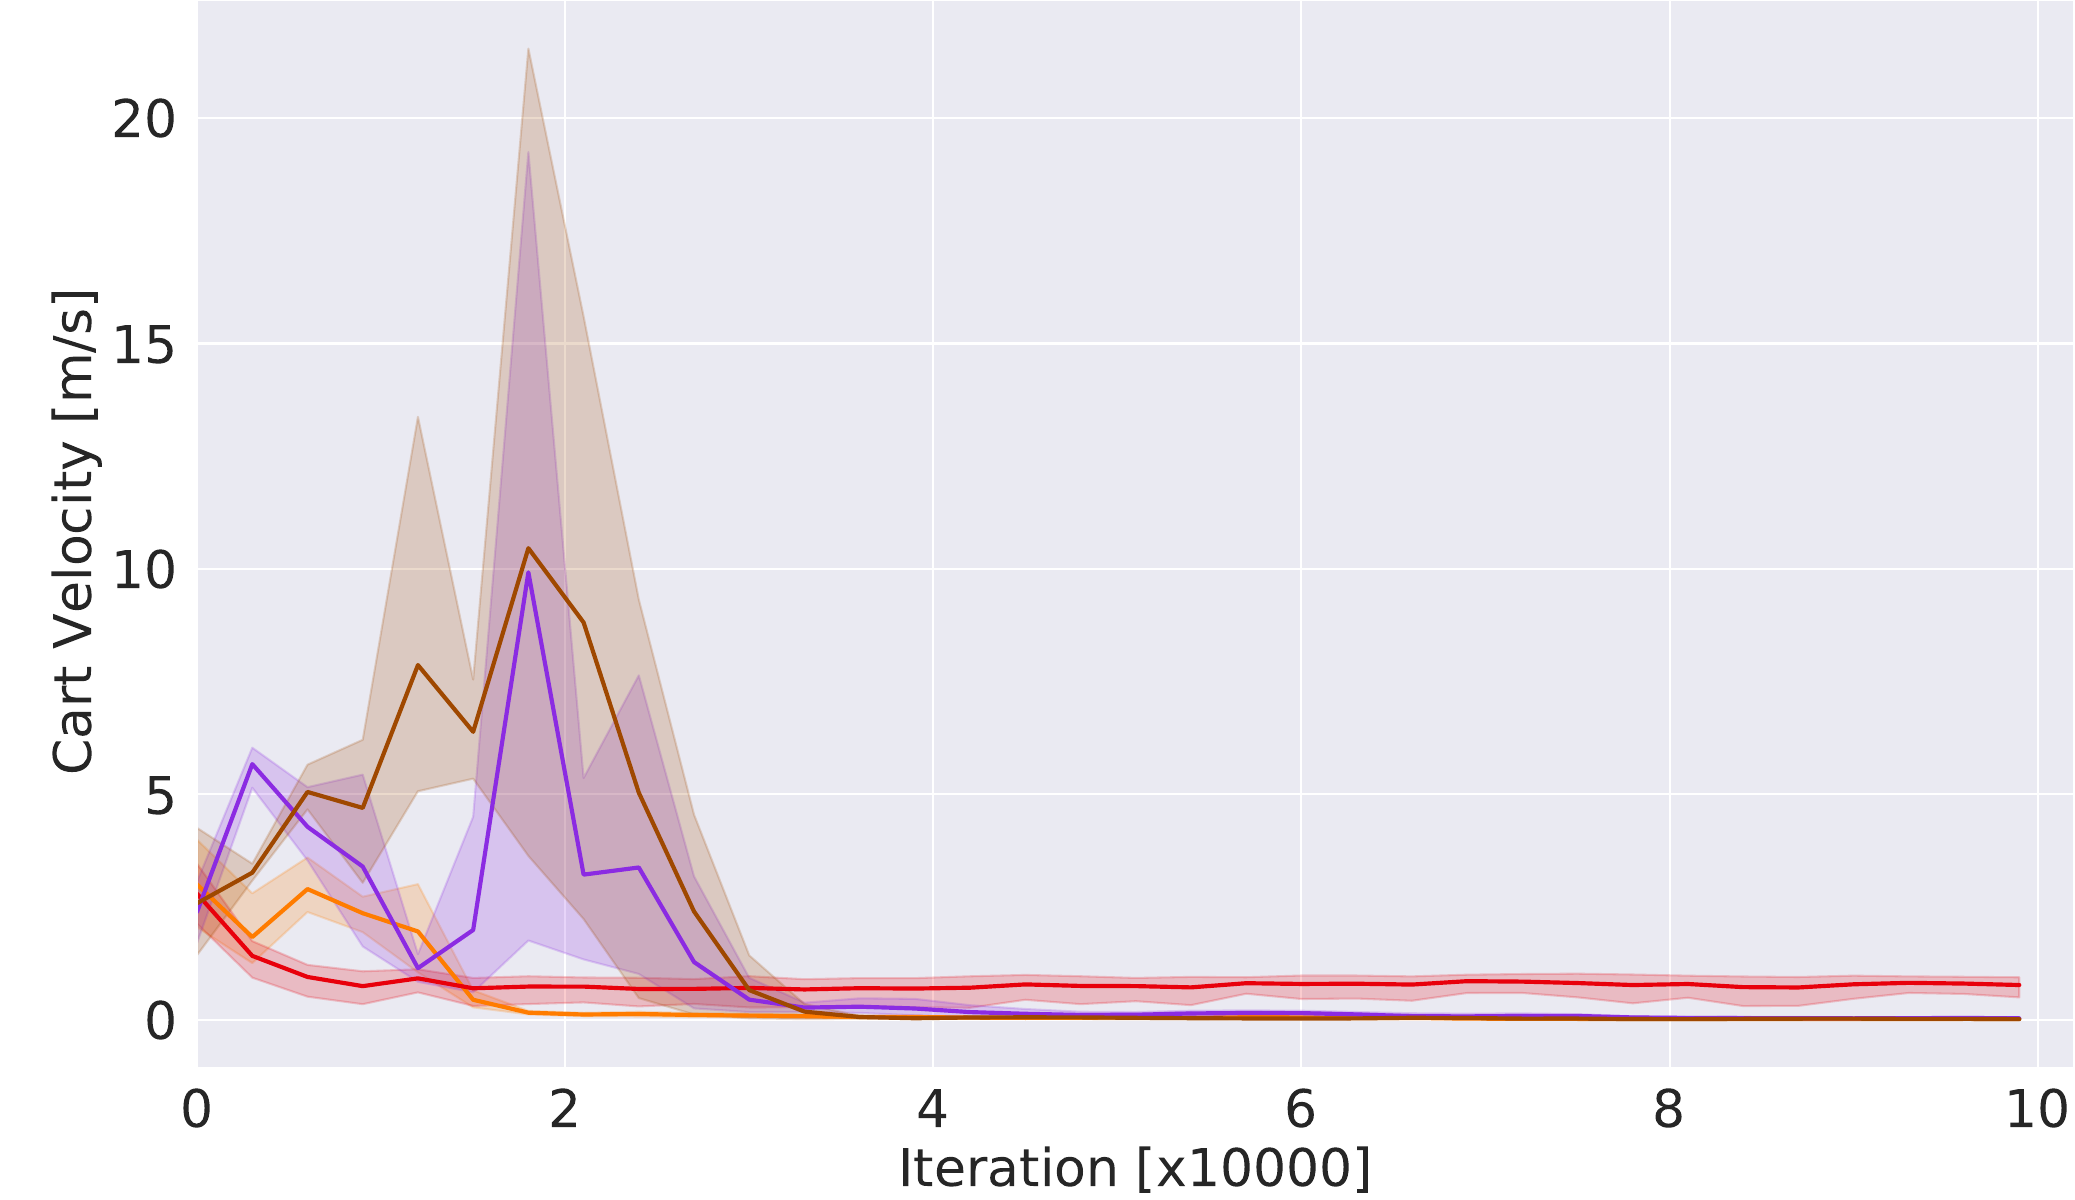}}\\
\subfloat[Pole angle]{\label{fig.pole_angle}\includegraphics[width=0.4\textwidth]{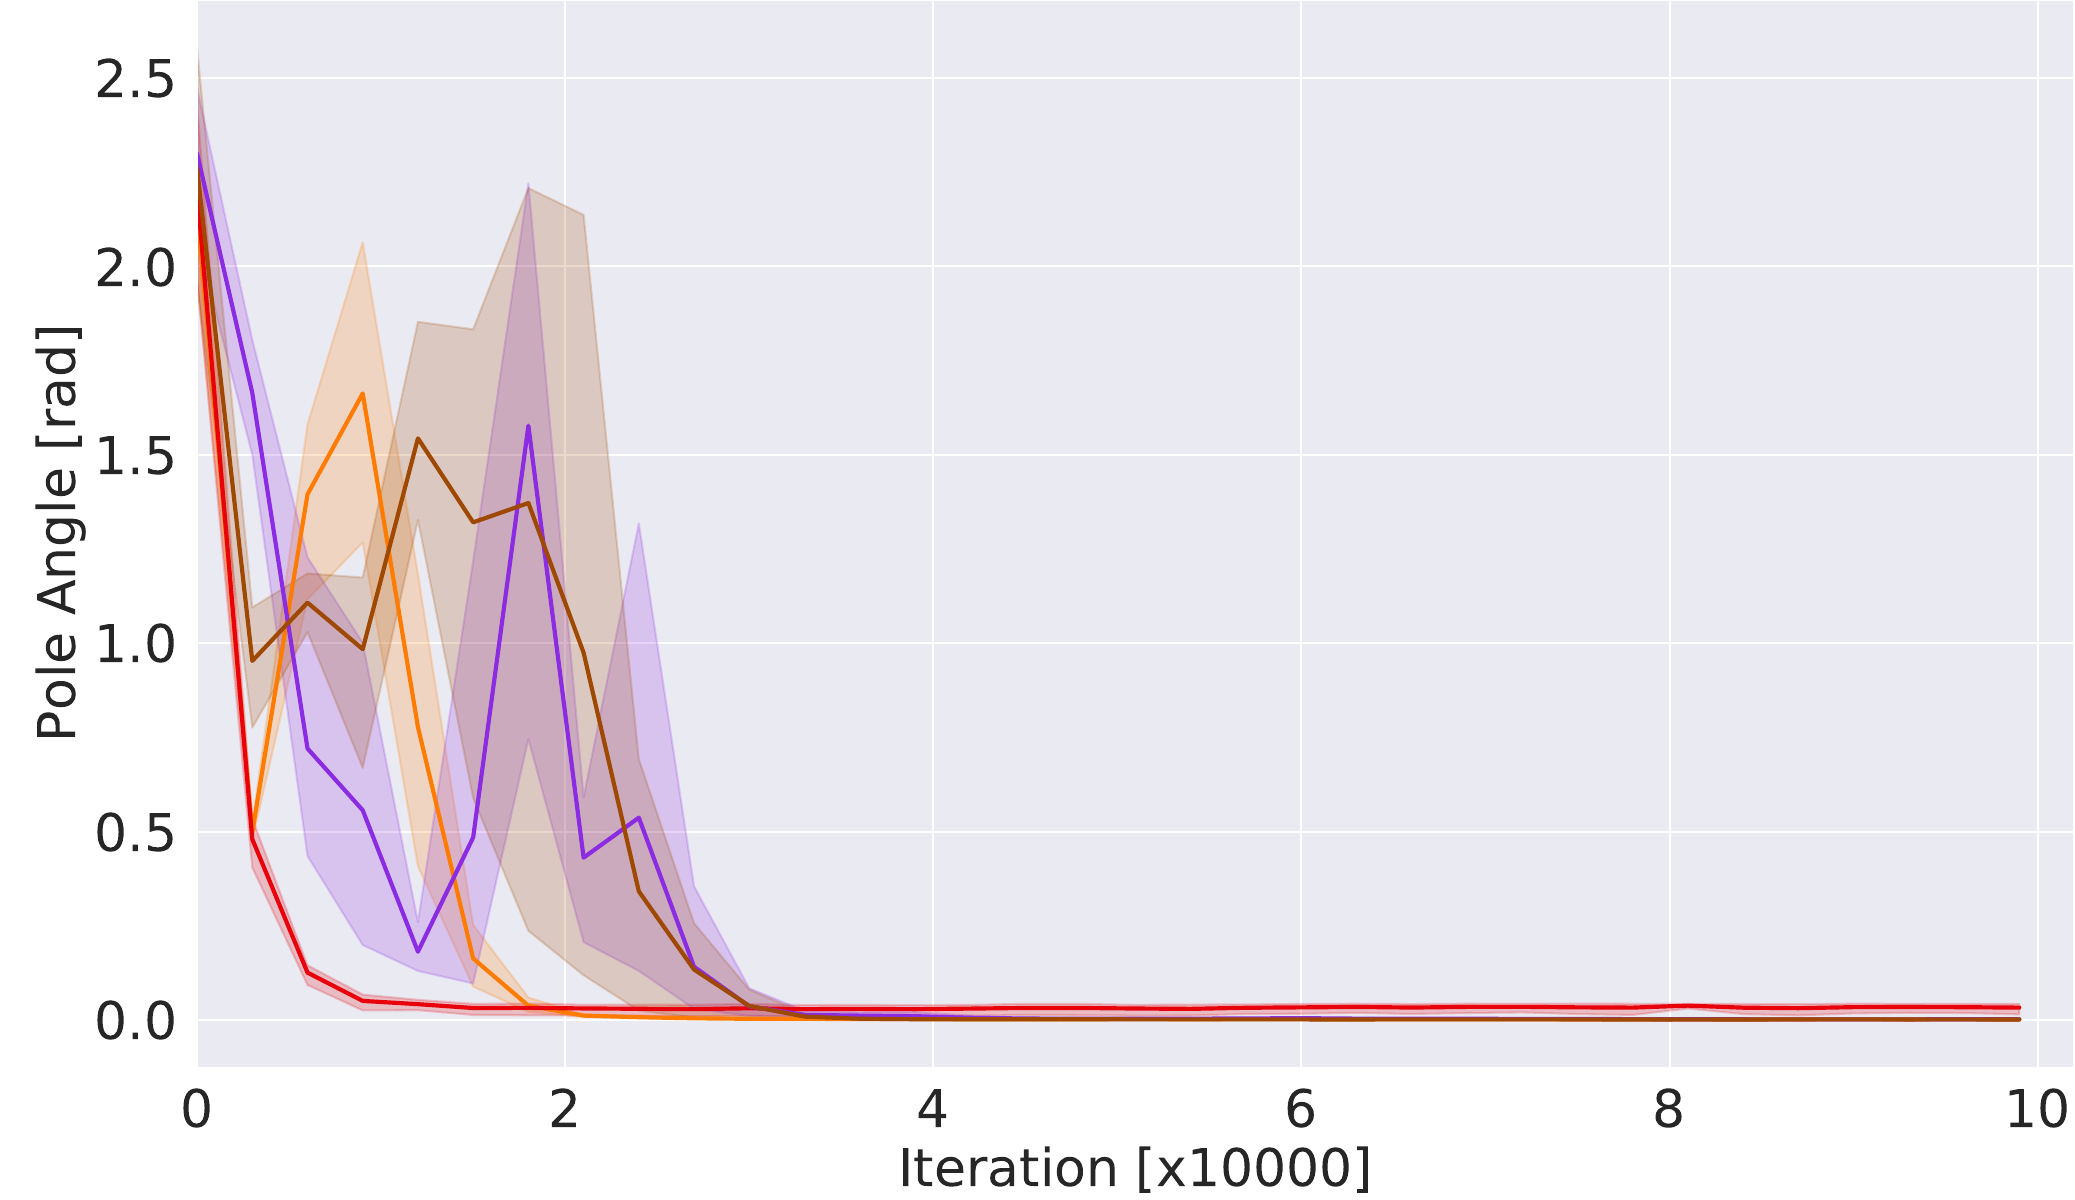}}\\
\subfloat[Pole angular velocity]{\label{fig.pole_angular_velocity}\includegraphics[width=0.4\textwidth]{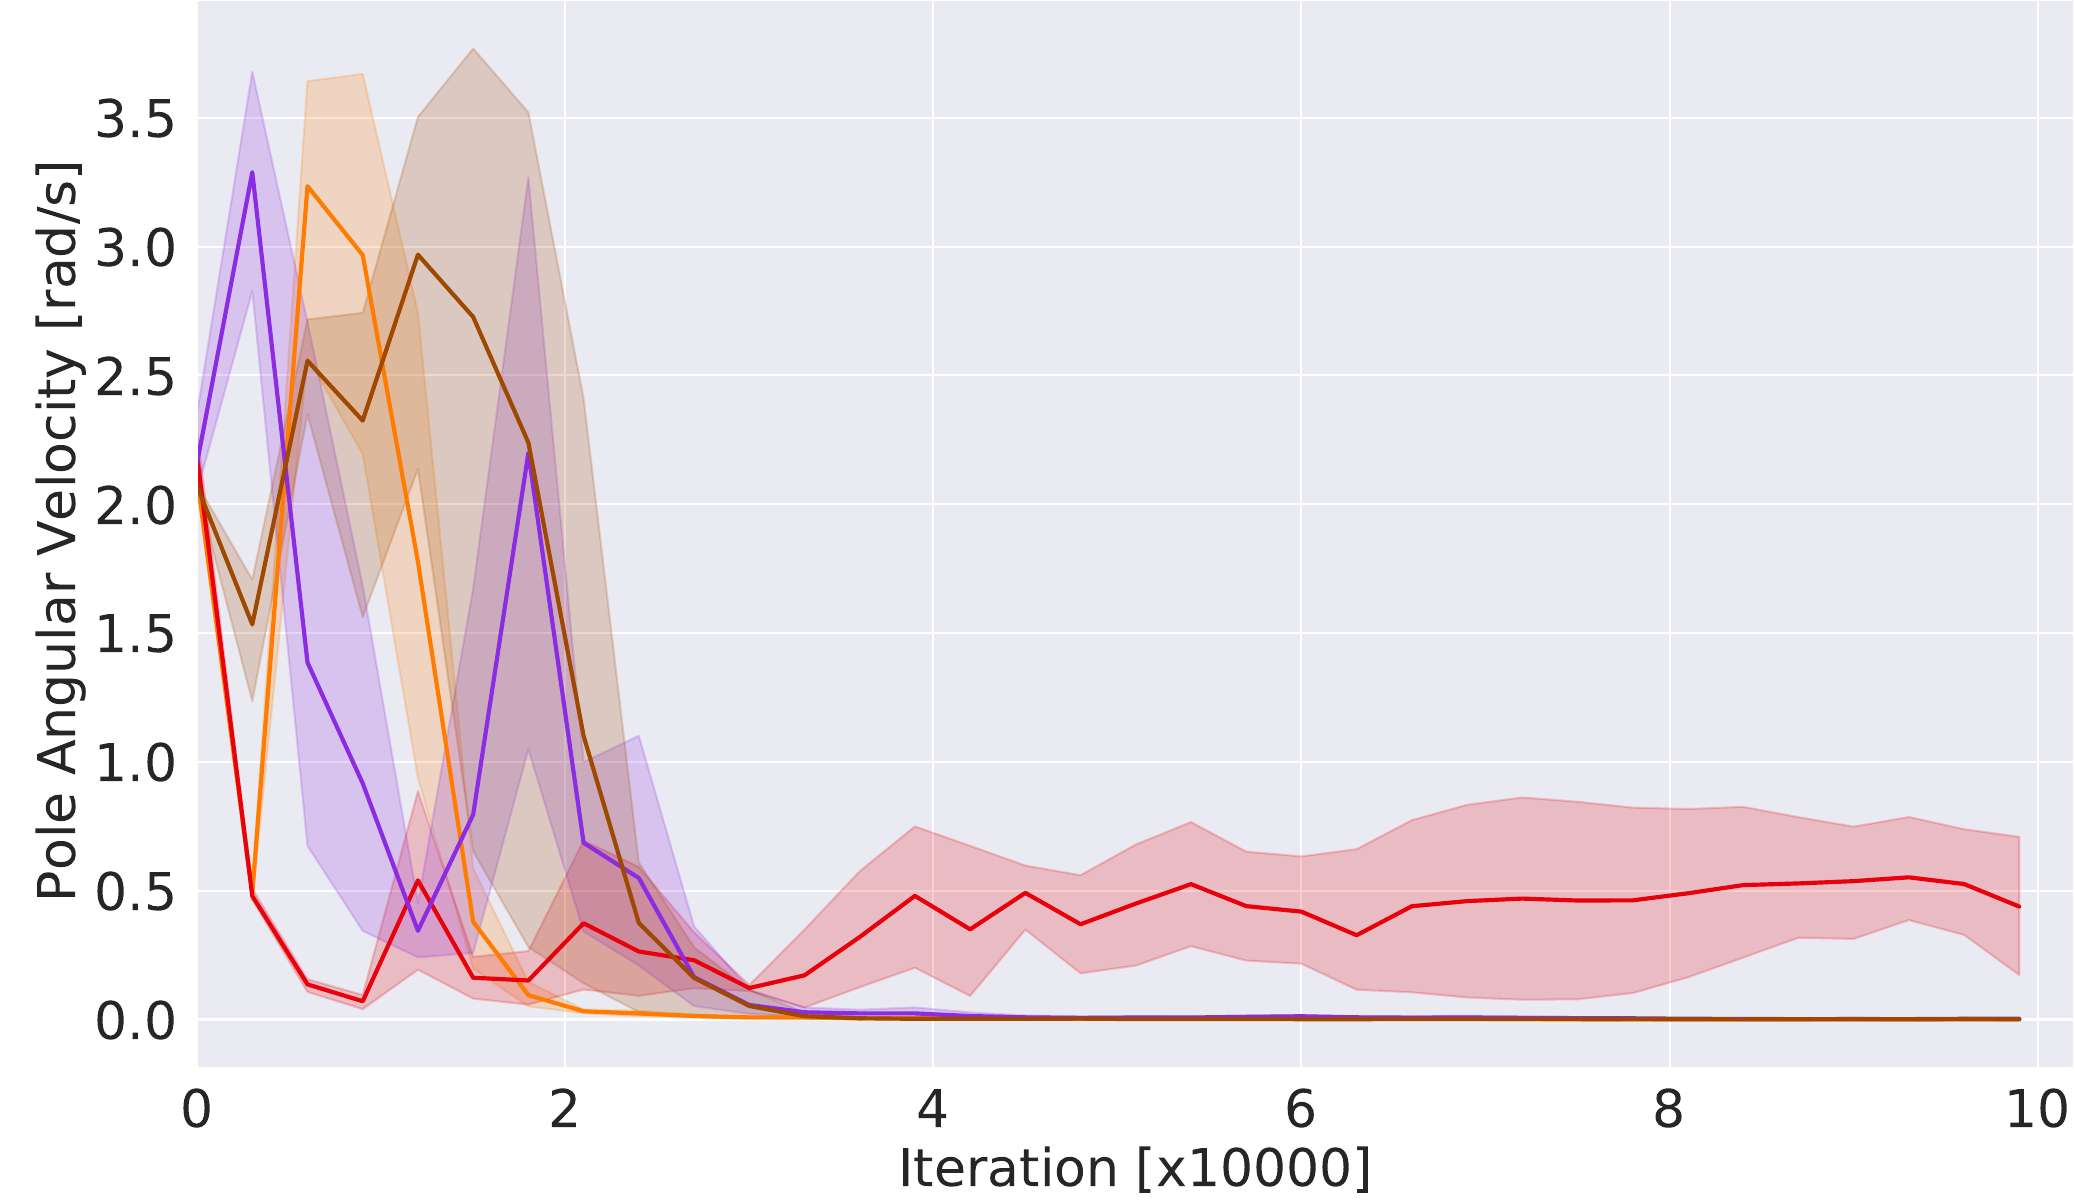}}
\caption{State magnitudes of inverted pendulum task. (a) Cart position. (b) Cart velocity. (c) Pole angle. (d) Pole angular velocity. The solid lines correspond to the mean and the shaded regions correspond to 95\% confidence interval over 5 runs.}
\label{fig.cart_pole_error}
\end{figure}
