# Supplementary material for: Mixed Policy Gradient: off-policy reinforcement learning driven jointly by data and model
Source: arXiv:2102.11513 source file (2024-02-24)
Supplement: Supplementary file 2 [file addi_descs.tex]

\section{Additional descriptions}\label{appendix.addi_desc}
