# Supplementary material for: Mixed Policy Gradient: off-policy reinforcement learning driven jointly by data and model
Source: arXiv:2102.11513 source file (2024-02-24)
Supplement: Supplementary file 3 [file baseline_algos.tex]

% \section{Baseline algorithms}\label{appendix.baseline_algs}
% \subsection{$n$-step DPG}\label{appendix.ndpg}
% Suppose the action-value function and policy are approximated by parameterized functions $Q_w(s, a)$ and $\pi_{\theta}(s)$ respectively. Given separate target action-value function $Q_{w'}$ and policy $\pi_{\theta'}$, the update target of $Q_{w}$ is calculated the same as MPG:
% \begin{equation}
% \nonumber
% R^{\text{Target}}(s, a) = \sum_{l=t}^{t+n-1} \gamma^{l-t} r_l + \gamma^{n} Q_{w'}(s_{t+n}, \pi_{\theta'}(s_{t+n})) \bigg|_{s_t=s, a_t=a}.
% \end{equation}
% where $s_{t+i} \sim p(\cdot|s_{t+i-1}, \pi_{\theta}(s_{t+i-1})), i \ge 1$;
% $r_{t+i} := r(s_{t+i}, \pi_{\theta}(s_{t+i})), i \ge 0$. The action-value function can be trained by directly minimizing
% \begin{equation}
% \nonumber
% J_Q(w) = \mathbb{E}_{s,a\sim \mathcal{B}}\left\{\frac{1}{2}(R^{\text{Target}}(s, a) - Q_w(s,a))^2\right\}.
% \end{equation}
% The policy can be learned by directly maximizing the learned action-value function, same as DPG:
% \begin{equation}
% \nonumber
% J_{\pi}(\theta) = \mathbb{E}_{s\sim \mathcal{B}}\left\{Q_w(s, \pi_{\theta}(s))\right\}.
% \end{equation}
% The pseudo-code of $n$-step DPG is shown in Algorithm \ref{alg.ndpg}.

% \begin{algorithm}[htbp]
%   \caption{$n$-step DPG}
%   \label{alg.ndpg}
% \begin{algorithmic}
%   \STATE {\bfseries Initialize:} critic network $Q_w$ and actor network $\pi_{\theta}$ with random parameters $w$, $\theta$, target parameters $w' \leftarrow w, \theta' \leftarrow \theta$, batch size $N$, initial buffer $\mathcal{B}$ with $N$ samples, exploration noise $\epsilon$, target smoothing coefficient $\tau$, learning rate $\beta_w, \beta_{\theta}$
%   \FOR{each iteration $k$}
%       \STATE Collect a batch of transitions using $\pi_{\theta}$ with noise $\epsilon$, store in $\mathcal{B}$
%       \STATE Sample $N$ transitions $\{s_i, a_i, r_i, s_{i+1}\}_{i=0:N-1}$ from $\mathcal{B}$
%       \STATE Update value $w \leftarrow w - \beta_w \nabla_{w}J_Q(w)$
%       \STATE Update policy $\theta \leftarrow \theta + \beta_{\theta} \nabla_{\theta}J_{\pi}(\theta)$
%       \STATE Update target networks:
%       \STATE \quad $w' \leftarrow \tau w + (1-\tau) w'$
%       \STATE \quad \ $\theta' \leftarrow \tau \theta + (1-\tau) \theta'$
%   \ENDFOR
% \end{algorithmic}
% \end{algorithm}

% \subsection{$n$-step ADP}\label{appendix.nadp}
% Suppose the action-value function and policy are approximated by parameterized functions $Q_w(s, a)$ and $\pi_{\theta}(s)$ respectively. Given separate target action-value function $Q_{w'}$ and policy $\pi_{\theta'}$, the update target of $Q_{w}$ is calculated as follows:
% \begin{equation}
% \nonumber
% R^{\text{Target}}(s, a) = \sum_{l=t}^{t+n-1} \gamma^{l-t} \hat{r}_l + \gamma^{n} Q_{w'}(\hat{s}_{t+n}, \pi_{\theta'}(\hat{s}_{t+n})) \bigg|_{\hat{s}_t=s, \hat{a}_t=a}.
% \end{equation}
% The action-value function can be trained by directly minimizing
% \begin{equation}
% \nonumber
% J_Q(w) = \mathbb{E}_{s,a\sim \mathcal{B}}\left\{\frac{1}{2}(R^{\text{Target}}(s, a) - Q_w(s,a))^2\right\}.
% \end{equation}
% The policy can be learned by directly maximizing $n$-step model return:
% \begin{equation}
% \nonumber
% J_{\pi}(\theta) = \mathbb{E}_{s\sim \mathcal{B}}\left\{\mathbb{E}_{\substack{\hat{s}_{t+1},\\ \dots, \\\hat{s}_{t+n}}}\left\{\sum_{l=t}^{n-1+t} \gamma^{l-t} \hat{r}_l + \gamma^{n} Q_{w, \hat{t+n}} \right\}\bigg|\hat{s}_t=s\right\}.
% \end{equation}
% where $\hat{s}_{t+i} \sim f(\cdot|\hat{s}_{t+i-1}, \pi_{\theta}(\hat{s}_{t+i-1})), i \ge 1$;
% $\hat{r}_{t+i} := r(\hat{s}_{t+i}, \pi_{\theta}(\hat{s}_{t+i})), i \ge 0$;  $Q_{w,\hat{t+i}}:=Q_w(\hat{s}_{t+i},\pi_{\theta}(\hat{s}_{t+i})), i \ge 1$. The pseudo-code of $n$-step ADP is shown in Algorithm \ref{alg.nadp}.

% \begin{algorithm}[htbp]
%   \caption{$n$-step ADP}
%   \label{alg.nadp}
% \begin{algorithmic}
%   \STATE {\bfseries Initialize:} critic network $Q_w$ and actor network $\pi_{\theta}$ with random parameters $w$, $\theta$, target parameters $w' \leftarrow w, \theta' \leftarrow \theta$, batch size $N$, initial buffer $\mathcal{B}$ with $N$ samples, target smoothing coefficient $\tau$, learning rate $\beta_w, \beta_{\theta}$
%   \FOR{each iteration $k$}
%       \STATE Collect a batch of transitions using $\pi_{\theta}$, store in $\mathcal{B}$
%       \STATE Sample $N$ transitions $\{s_i, a_i, r_i, s_{i+1}\}_{i=0:N-1}$ from $\mathcal{B}$
%       \STATE Update value $w \leftarrow w - \beta_w \nabla_{w}J_Q(w)$
%       \STATE Update policy $\theta \leftarrow \theta + \beta_{\theta} \nabla_{\theta}J_{\pi}(\theta)$
%       \STATE Update target networks:
%       \STATE \quad $w' \leftarrow \tau w + (1-\tau) w'$
%       \STATE \quad \ $\theta' \leftarrow \tau \theta + (1-\tau) \theta'$
%   \ENDFOR
% \end{algorithmic}
% \end{algorithm}
